# Supplementary material for: Understanding Time Variations of DNN Inference in Autonomous Driving
Source: arXiv:2209.05487 source file (2022-09-12)
Supplement: Supplementary file 1 [file 8_appendix.tex]

\label{appendix}
